# Supplementary material for: Accelerating Grasp Exploration by Leveraging Learned Priors
Source: arXiv:2011.05661 source file (2020-11-11)
Supplement: Supplementary file 1 [file 8-appendix.tex]

\newpage
\appendix
\section{Proofs}
\subsection{Proof of \Cref{thm:prob-miss-pose}}
We can prove this claim by induction. For the base case, consider $T = 1$. In this case it is easy to see that $p^\pi_1(P^i) = \lambda_i$ since the probability of encountering stable pose $P^i$ within one round of learning is simply the probability that the object is initially dropped into stable pose $P^i$.

For the inductive step, assume that 
\begin{align*} 
\begin{split}
p^\pi_{T-1}(P^i) = \lambda_i \left[ 1 + \sum_{k=2}^{T-1} \sum_{j=2}^{k} {k-2 \choose j-2} \left[ (1 - \lambda_i)\eta^\pi_i \right]^{j-1} \left[1 - \eta^\pi_i\right]^{k-j}\right]
\end{split}
\end{align*}
The induction hypothesis captures the probability that stable pose $P^i$ has been encountered within the first $T-1$ rounds, so to perform the inductive step, we must compute the probability that stable pose $P^i$ is first encountered on round $T$. The sum of these probabilities is simply the probability $p^\pi_{T}(P^i)$ that stable pose $P^i$ is encountered within the first $T$ rounds as desired.

We can compute the probability that $P^i$ is first encountered on round $T$ as follows. The probability of observing a stable pose other than $P^i$ on round 1 is simply $1 - \lambda_i$. Now we consider the set of possible transitions from this initial stable pose. There are three cases to consider: (1) if the object is not successfully grasped, the object is guaranteed to not be in the same stable pose on the next timestep; if the object is successfully grasped, (2) the object will not be in pose $P_i$ on the next timestep with probability $1 - \lambda_i$ and (3) will be in pose $P^i$ on the next timestep with probability $\lambda_i$. Thus, given that the object is not in stable pose $P^i$, cases (1) and (2) guarantee that the object will continue not to be in stable pose $P^i$ on the next timestep while case (3) guarantees that it will be in stable pose $P^i$ on the next timestep. Thus, we compute the probability of all possible $T$-length sequences in which cases (1) and (2) occur for the first $T-1$ timesteps and case (3) occurs at timestep $T$.

At each timestep, case (1) occurs with probability $1 - \eta^\pi_i$, case (2) occurs with probability $\eta^\pi_i (1 - \lambda_i)$ and case (3) occurs with probability $\eta^\pi_i \lambda_i$. To ensure that the object stays in pose other than $P^i$ for the first $T-1$ timesteps and then transitions into $P^i$ on timestep $T$, it must be the case that the object falls into a stable pose other than $P^i$ on round 1, that for the next $T-2$ timesteps, either cases (1) or (2) occur, and that case (3) occurs on timestep $T$. We can simply compute this by summing up the probability of all such sequences as follows:
\begin{align*} 
\begin{split}
(1 - \lambda_i){T - 2 \choose 0} \left[  (1 - \eta^\pi_i) \right]^{T-2}& \left[  (1 - \lambda_i)\eta^\pi_i \right]^{0} \left(\eta^\pi_i \lambda_i\right) + \\
(1 - \lambda_i){T - 2 \choose 1} \left[  (1 - \eta^\pi_i) \right]^{T-3}& \left[  (1 - \lambda_i)\eta^\pi_i \right]^{1} \left(\eta^\pi_i \lambda_i\right) + \\ 
&\vdots \\
(1 - \lambda_i){T - 2 \choose T - 2} \left[  (1 - \eta^\pi_i) \right]^{0}& \left[  (1 - \lambda_i)\eta^\pi_i \right]^{T-2} \left(\eta^\pi_i \lambda_i\right) 
\end{split}
\end{align*}

Note that this can be written as 
\begin{align*}
\begin{split}
(1 - \lambda_i)\eta^\pi_i\lambda_i \sum_{j = 2}^{T} {T-2 \choose j - 2} \left[ (1 - \lambda_i)\eta^\pi_i \right]^{j-2} \left[1 - \eta^\pi_i\right]^{T - j}\\
= \lambda_i \sum_{j = 2}^{T} {T-2 \choose j - 2} \left[ (1 - \lambda_i)\eta^\pi_i \right]^{j-1} \left[1 - \eta^\pi_i\right]^{T - j}
\end{split}
\end{align*}

Adding this to the induction hypothesis gives the desired result. \qed

\subsection{Proof of \Cref{cor:prob-miss-pose}}
Since $p^\pi_{T}(P^i)$ gives the probability of encountering a stable pose $P^i$ within $T$ timesteps, $1 - p^\pi_{T}(P^i)$ gives the probability of never encountering $P^i$ in the first $T$ timesteps. To obtain the probability of never encountering a stable pose with drop probability $\lambda_i$, we simply substitute $\lambda_i = \epsilon$ into the expression for $1 - p^\pi_{T}(P^i)$ and the result immediately follows. \qed

\subsection{Proof of \Cref{thm:regret-bound}}
Theorem 2 from~\cite{TS-regret} establishes that for the $K$-armed stochastic bandit problem, Thompson sampling using Beta priors achieves expected total regret in time $T$ which is bounded above as follows.
\begin{align}
    \label{eq:regret-bound}
     \mathbb{E}\left[\mathcal{R}(T)\right] = \mathcal{O}(\sqrt{KT \ln T}) 
\end{align}

Thus, $\mathbb{E}\left[\mathcal{R}(T)\right] \leq M \sqrt{KT \ln T}$ for some $M > 0$ and sufficiently large $T$. Thus, we can apply this result to bound the expected total regret for grasp exploration on any given pose $P^l$ defined in \Cref{def:regret} as follows:
\begin{align}
    \label{eq:regret-bound-stable-pose}
\mathbb{E}\left[\mathcal{R}_{P^l}(T_l)\right] \leq M \sqrt{KT_l \ln T_l}
\end{align}

Direct application of the definition of the regret over all stable poses from \Cref{def:pose-regret} yields the desired result. \qed

\section{Additional Method Details}

\section{Additional Experimental Results}
